# Supplementary material for: Mixed Diffusion for 3D Indoor Scene Synthesis
Source: arXiv:2405.21066 source file (2024-12-09)
Supplement: Supplementary file 1 [file scene_completion_additional.tex]

%!TEX root = ../main.tex

% floor conditioned layout synthesis with existing objects - additional results

\begin{table}[ht]
\vspace{-0.2cm}
\resizebox{\textwidth}{!}{
\begin{tabular}{llcccclcccclcccc}
\hline
\multirow{2}{*}{Method} &  & \multicolumn{4}{c}{Bedroom}  &  & \multicolumn{4}{c}{Dining room} &  & \multicolumn{4}{c}{Living room} \\ \cline{3-6} \cline{8-11} \cline{13-16} 
            &  & FID   &KIDx0.001& CA \%   &KLx0.01&  & FID   &KIDx0.001& CA \%   &\small{KLx0.01}&  & FID   &KIDx0.001& CA \%   &KLx0.01\\ \hline
ATISS       &  & 51.83          & -0.57 & 56.89 +/- 3.86          & \textbf{0.66}          &  & 33.53          & 5.39          & 55.31 +/- 4.54          & 1.60          &  & 31.78          & 5.39          & 59.53 +/- 4.78          & 1.43          \\
DiffuScene  &  & \textbf{42.77} & \textbf{-1.08} & \textbf{52.26 +/- 1.10} & 0.80          &  & 30.58          & 3.67          & 53.67 +/- 4.35          & \textbf{0.84} &  & 32.07          & 4.58          & 59.80 +/- 4.38          & \textbf{0.57} \\
\algorithm(Ours)        &  & 51.87          & -0.34 & 57.44 +/- 4.01    & 0.70      &  & \textbf{28.01} & \textbf{2.03} & \textbf{52.57 +/- 3.10} & 1.72          &  & \textbf{28.74} & \textbf{1.97} & \textbf{57.60 +/- 4.31} & 0.97         \\
 \hline
\end{tabular}
}
\caption{Evaluation results for scene completion given 3 existing objects. \label{tab:scene_completion}} 
% \vspace{-0.4cm}
\end{table}
